# Supplementary material for: Towards Motion Turing Test: Evaluating Human-Likeness in Humanoid Robots
Source: arXiv:2603.06181 source file (2026-03-06)
Supplement: Supplementary file 1 [file supplementary.tex]

\clearpage
\setcounter{page}{1}

\twocolumn[{
\renewcommand\twocolumn[1][!htb]{#1}
\maketitlesupplementary
% \vspace{-10mm}
\begin{center}
    \centering
    \includegraphics[width=1\linewidth]{figs/data_stas2.png}
    \vspace{-6mm}
    \captionof{figure}{\textbf{HHMotion dataset.} The left table summarizes the full data composition,  
    including all collection sources spanning real-world humanoid robots, simulated environments, and human motion recordings. 
    The right lists every humanoid robot included in HHMotion.
    % , covering a diverse range of manufacturers to ensure broad representativeness of current humanoid motion capabilities.
}
    \label{fig:data_stas}
    % \vspace{-1mm}
\end{center}
}]

% \maketitlesupplementary

% \begin{figure*}[t]
%     \centering
%     \includegraphics[width=1\linewidth]{figs/data_stas.png}
%     \caption{Overview of the HHMotion dataset sources and humanoid robot models}
%     \label{fig:data_stas}
% \end{figure*}

Thanks for reading the supplementary. In this supplementary file, we provide additional technical details for the Evaluating Human-Likeness in Humanoid Robots framework. 
Moreover, a demo video is included in the supplementary to illustrate the overall pipeline and showcase representative evaluation examples.

\section{More Details on HHMotion Dataset}

\subsection{Dataset Composition and Sources}
\subsubsection{HHMotion dataset sources}
%Detailed description of HHMotion dataset sources. 
The HHMotion dataset integrates motion data from a wide spectrum of human and humanoid behaviors to construct a unified benchmark for evaluating human-likeness. It comprises five complementary motion sources, each contributing distinct characteristics and distribution patterns: 

\begin{figure}[t]
    \centering
    \includegraphics[width=1\linewidth]{figs/4action_example1.png}
    \caption{Representative examples of human and humanoid robot motions across four action categories. Full visualizations of all 15 categories are provided on the last page of the supplementary.}
    \label{fig:4example}
\end{figure}

\begin{figure*}[t]
    \centering
    \includegraphics[width=1\linewidth]{figs/data_sanitation2.png}
    \caption{\textbf{The Data Sanitation Pipeline of HHMotion.} We illustrate the rigorous multi-stage pipeline used to construct the dataset from over 21 hours of raw footage.}
    \label{fig:data_sanitation}
\end{figure*}

1) Real-World Humanoid Robots.
Videos were collected from major public events and online releases of state-of-the-art humanoid robots in 2025. The public international events include the World Artificial Intelligence Conference (WAIC)~\cite{waic2025}, World Robot Conference (WRC)~\cite{wrc2025}, World Humanoid Robot Games (WHRG)~\cite{whrg2025}, which represent the current state of the art in humanoid robotics. These sequences capture genuine hardware constraints such as mechanical latency, limited joint ranges, ground interaction noise, and stability control behaviors. 

2) Simulated Humanoid Robots.
To expand the diversity of robot motions, we include high-quality simulated sequences. These clips often exhibit smoother trajectories and reduced noise compared to real robots, providing a valuable contrast for analyzing comprehensive discrepancies in human-likeness score.

3) Human Motions from Volunteers.
Ten subjects with varied movement habits performed the same set of action categories as the robots. These sequences serve as the reference for natural human movement, capturing subtle cues such as inertia continuity and posture fluidity.

4) Humans Imitating Humanoid Robots subset.
To introduce ambiguous and challenging cases for human-likeness evaluation, the volunteers also performed robot motions. Participants mimic the stiffness of humanoid robots. These sequences blur the boundary between human and robotic motion and increase the challenge of evaluation scenarios.

5) Additional Human motions from YouTube.
To further enhance diversity, we curate additional human action videos from YouTube, covering a range of performance styles and outdoor scenes. These samples enrich motion variety and help prevent overfitting to controlled laboratory environments.

Across these five sources, HHMotion incorporates 11 distinct humanoid robot models, as shown in Fig.~\ref{fig:data_stas}, offering a comprehensive foundation for evaluating human-likeness in motion dataset.

%A detailed list of the humanoid robot models included in the dataset.把那个机器人型号的图放上来。

\subsubsection{Motion Categories in HHMotion}

% The HHMotion dataset spans 15 diverse action categories, designed to capture a wide range of full-body dynamics, lower-limb, and upper-limb movement complexities crucial for human-likeness evaluation. The categories include \textit{boxing, dance, jump, kungfu, run, gymnastics, fall and get up, fight, ski, ping pong, waving, walk, kicking ball, sit, and stand.} Fig.~\ref{fig:15action_humanoid} shows the 15 motion categories for humanoid robots, and Fig.~\ref{fig:15action_human} shows the corresponding 15 motion categories for humans. 
The HHMotion dataset spans 15 diverse action categories covering full-body, lower-limb, and upper-limb motion patterns essential for assessing human-likeness. In this section, we present only four representative categories to illustrate the contrast between human and humanoid motion in Fig.~\ref{fig:4example}. The complete visualization of all 15 action categories for both humans and humanoid robots is provided in Fig.~\ref{fig:15action_humanoid} and Fig.~\ref{fig:15action_human}. 

These 15 motion categories jointly cover slow, fast, cyclic, and fine-grained limb actions, ensuring that the dataset captures a broad spectrum of kinematic characteristics essential for measuring human-likeness across both humans and humanoid robots.

\subsection{Data Sanitation Pipeline}
% Noise Filtering
% 移除低分辨率、严重遮挡、裁剪不完整的视频
% 移除亮度不足、运动模糊、高压缩伪影片段
% Temporal Trimming
% 手动 + 自动定位动作周期
% 切成统一的 5 秒动作片段
% Pose Validation
% 使用 SMPL-X 重建
% 排除重建失败、关键帧跳动（tracking jitter）
% Human-Humanoid Balance Enforcement
% 选取等量的人类与机器人的动作片段
% 保证动作类别分布平衡
% 最终得到约 5,000 秒高质量片段（1,000 clips）

% To ensure high-quality and reliable motion data, we perform a multi-stage sanitation pipeline on all raw videos. First, we conduct noise filtering by removing segments with low resolution, severe occlusion, incomplete cropping, motion blur, or heavy compression artifacts. Next, temporal trimming is used to identify valid action cycles and edit each sample into a 5-second motion clip. We then perform pose validation using SMPL-X reconstruction, discarding any sequences exhibiting reconstruction failures, tracking jitter, or implausible poses. Finally, we enforce a strict human–humanoid balance by selecting equal volumes of clips across both sources to keep the action distribution consistent. After this sanitation pipeline, we obtain approximately 5,000 seconds of clean motion data (about 1,000 high-quality clips) for evaluation. The pipeline of data sanitation is shown in Fig.~\ref{fig:data_sanitation}.

To ensure the reliability of the benchmark and address the domain gap challenge when generalizing HPE methods to humanoid robots, we implemented a rigorous, multi-stage data sanitation pipeline. Starting with over 21 hours of raw footage, we processed the data through the steps as shown in Fig.~\ref{fig:data_sanitation}.

\textbf{1) Visual Quality Filtering and Standardization.} 
% First, we conducted strict \textbf{noise filtering} on the raw video corpus. Segments exhibiting low resolution, severe occlusion, incomplete subject cropping, or significant motion blur were systematically discarded to ensure visual clarity. Following this, we performed manual \textbf{temporal trimming} to standardize the temporal duration of actions. Each valid action cycle was carefully segmented into a unified 5-second motion clip, ensuring semantic completeness and temporal consistency across the dataset.
We first performed strict \textbf{noise filtering} over the entire 21-hour raw corpus. Videos exhibiting low resolution, severe occlusion, incomplete subject cropping, strong compression artifacts, or motion blur were removed. This stage eliminated a substantial portion of low-quality content, resulting in approximately \textbf{5 hours} of visually reliable videos. We then conducted manual \textbf{temporal trimming} on this 5-hour subset to extract semantically complete action cycles. Each identified motion segment was normalized to a uniform 5-second duration, producing a pool of \textbf{1,110 candidate clips} across both human and humanoid sources.

\textbf{2) Rigorous Pose Validation via Manual Inspection.} 
% A critical challenge in our pipeline is ensuring that HPE methods designed for humans (e.g., GVHMR) generalize effectively to humanoid robots. To address this, we employed a strict \textbf{pose validation} stage involving manual cross-validation. We first reconstructed SMPL-X sequences for an initial \textbf{candidate of 610} humanoid motion clips. We then manually inspected each SMPL-X sequence frame-by-frame to identify artifacts arising from the domain shift, such as tracking jitter, reconstruction failure, or physiologically implausible poses. Through this rigorous screening, we \textbf{filtered out 110 low-quality}  sequences, retaining only the top 500 high-quality humanoid clips that demonstrated stable and accurate kinematic reconstruction.
A major challenge lies in ensuring that human-oriented HPE models (e.g., GVHMR) generalize reliably to humanoid robots. To mitigate domain-shift artifacts, we applied a strict \textbf{pose validation} stage to all 1,110 candidate clips. We reconstructed SMPL-X poses for every clip and performed frame-by-frame manual inspection to detect common failure cases, including tracking jitter, mesh distortions, and physiologically implausible poses. 
% Clips affected by such issues were discarded. After this rigorous validation, we retained \textbf{500 high-quality humanoid clips} and an equal number of high-quality human clips for downstream evaluation. 
Following this quality screening, we strictly enforced \textbf{class balance} to prevent evaluation bias. We retained the top \textbf{500 high-quality humanoid clips} that passed inspection and matched them with an equal volume of verified high-quality human clips. This process ensures a consistent action distribution across both domains while guaranteeing that all included sequences demonstrate stable kinematic reconstruction. Please refer to details regarding the HPE methods in Sec.~\ref{sec:hpe}.

% \textbf{3) Human–Humanoid Balance Enforcement.} Finally, to prevent class imbalance bias during evaluation, we applied \textbf{balance enforcement}. We matched the retained 500 humanoid clips with an equal volume of high-quality human motion clips, ensuring a consistent action distribution across both domains.

After this comprehensive sanitation pipeline, we obtained approximately 5,000 seconds of clean, high-quality motion data (comprising 1,000 clips), establishing a robust foundation for the Motion Turing Test.

\subsection{Data Processing and Pose Estimation}\label{sec:hpe}
%Detailed comparison and experimental results of the SOTA Human Pose Estimation (HPE) methods evaluated.
%人类交叉验证，留下质量高的smplx
To obtain reliable 3D body parameters for all clips in HHMotion, we establish a unified data processing pipeline centered on SMPL-X reconstruction. Multiple state-of-the-art (SOTA) Human Pose Estimation (HPE) models are evaluated, and only high-quality reconstructions are retained through human cross-validation.
\begin{figure}[t]
    \centering
    \includegraphics[width=0.7\linewidth]{figs/adjust_bbx.png}
    \caption{\textbf{Manual Adjustment of Bounding Boxes.} Illustration of the effect of manual correction on automatically detected bounding boxes. The upper shows raw detector outputs, which may include loose framing. The lower shows manually refined bounding boxes that ensure tighter alignment with the humanoid.}
    \label{fig:adjust_bbx}
\end{figure}

\subsubsection{Manual Bounding Box Adjustment}
%description of the manual bounding box refinement process to improve HPE tracking quality.（个例讨论）
Although modern HPE pipelines include automated person detection, raw detections often suffer from loose boxes, missing extremities, or frame-to-frame jitter, which can significantly degrade downstream SMPL-X fitting quality. To address these issues, we incorporate a refinement stage using the CVAT~\cite{CVAT} annotation platform for efficient bounding-box correction. Annotators adjust boxes only on frames where automated detection clearly fails, such as rapid limb motion causing partial cropping, humanoid robot structures confusing the detector, or multi-person scenes leading to identity switches. This targeted correction ensures stable and consistent tracking across all clips while keeping annotation costs manageable. The tracking effect before and after optimizing the bounding box is shown in Fig.~\ref{fig:adjust_bbx}.

\begin{figure}[t]
    \centering
    \includegraphics[width=1\linewidth]{figs/skeleton1.png}
    \caption{\textbf{Annotated humanoid key joints for SMPL-X evaluation.}  
Representative examples of the 2D skeletal annotations used to assess SMPL-X reconstruction quality on humanoid robots.}
    \label{fig:skeleton}
\end{figure}

\begin{table}[t]
\centering
% \small
\caption{\textbf{Comparison of state-of-the-art HPE methods on our annotated robot motion set.} GVHMR is chosen as the SMPL-X reconstruction method for HHMotion since it achieves the lowest MPJPE and PAMPJPE (Unit: \textit{pixel}).}
\resizebox{\linewidth}{!}{
\begin{tabular}{l|ccc}
\toprule
\textbf{Method} & \textbf{MPJPE} $\downarrow$ & \textbf{PAMPJPE} $\downarrow$ & \textbf{PCK@0.3} $\uparrow$ \\
\midrule
TRACE~\cite{sun2023trace}        &  64.30  &  39.47  &  0.9384  \\
WHAM~\cite{shin2024wham}          & 66.13  &  28.42  &  0.9283  \\
PromptHMR~\cite{wang2025prompthmr}\        & 57.73  & 25.38  & 0.9150  \\
\midrule
\textbf{GVHMR}~\cite{shen2024world} & \textbf{28.23} & \textbf{25.33} & \textbf{0.9925} \\
\bottomrule
\end{tabular}
}
\label{tab:hpe_comparison}
% \vspace{-2mm}
\end{table}

\subsubsection{Comparison results of the HPE methods}
%Extended quantitative comparison of SMPL-X reconstruction performance across several SOTA Human Pose Estimation (HPE) methods.
To systematically evaluate the robustness of existing SMPL-X reconstruction methods on humanoid robots, we curated 50 representative robot videos in the HHMotion dataset. For each video, annotators manually labeled \textbf{14 key joints} using CVAT~\cite{CVAT}, including the \textbf{nose, neck, shoulders, elbows, wrists, hips, knees, and ankles,} to provide a ground-truth 2D skeletal reference for evaluating pose accuracy in humanoid. Fig.~\ref{fig:skeleton} shows the representative examples of the labeled humanoid's 14 key joints.

Using these keypoint annotations, we tested several SOTA SMPL-X recovery methods and computed standard metrics such as MPJPE and PAMPJPE. The experimental results are shown in Tab.~\ref{tab:hpe_comparison}. The comparison shows that most HPE methods exhibit varying degrees of degradation on humanoid robots due to non-human limb proportions, rigid body articulation, or reflective materials. Among all evaluated methods, GVHMR~\cite{shen2024world} demonstrates the most stable performance, achieving the lowest MPJPE and the most consistent reconstruction across different robot forms. This method is therefore adopted as the primary SMPL-X reconstruction backend for the HHMotion dataset.

\subsection{Annotation Quality and Analysis}
%The Inter-Annotator Consistency (IAC) check process (formulation) and its analysis results.
% Details of annotator consistency analysis, including:
% Inter-Annotator Consistency (IAC) formulation
% statistical result
% To ensure the reliability of the human-likeness annotations in HHMotion, we performed a comprehensive Inter-Annotator Consistency (IAC) analysis over all 30 annotators as shown in Alg.~\ref{alg:iac_algo}. Each annotator rated 1000 clips, and their scores were compared against the aggregated consensus rating. We evaluated two complementary measures: the Mean Squared Error (MSE), which captures absolute deviation from consensus, and Spearman’s rank correlation coefficient, which reflects the consistency of relative ordering. Annotators exceeding the MSE threshold or falling below the correlation threshold were considered unreliable, and those violating both were classified as high-risk.

% The analysis identified 5 annotators as high-risk with simultaneously large MSE ($\ge$ 1.41) and low correlation($\le$ 0.50). The remaining 25 annotators demonstrated acceptable reliability and were retained. As shown in Tab.~\ref{tab:iac_summary}, the overall annotation quality improved noticeably after filtering, with the mean MSE decreasing from 1.1817 to 0.9764 and the mean correlation increasing from 0.5215 to 0.5457. These results confirm that the IAC filtering step effectively reduces noise and enhances the stability of human-likeness supervision.

In this work, we invited 30 volunteers to annotate the motion human-likeness score for each clip. To ensure the reliability of human-likeness annotations in HHMotion, we conducted a rigorous Inter-Annotator Consistency (IAC) analysis across all 30 annotators, following best practices widely adopted in \textbf{psychometrics}, \textbf{subjective quality assessment}, and \textbf{human rating studies}~\cite{Shrout_1979, thurstone2017law, series2012methodology, snow2008cheap, raykar2010learning}.
These communities routinely rely on error-to-consensus deviation (e.g., MSE) combined with rank-based agreement metrics (e.g., Spearman $\rho$) to quantify rating stability, especially for subjective perceptual judgments where absolute values and relative ordering are both meaningful.

In our setup, each annotator rated 1,000 clips. As shown in Alg.~\ref{alg:iac_algo}, we first computed the consensus trajectory by taking the clip-wise mean score, which is a standard and statistically robust aggregation strategy when the number of annotators is sufficiently large. We then evaluated each annotator using two complementary reliability indicators:
\begin{itemize}
    \item \textbf{Absolute Deviation (MSE):} We compute the Mean Squared Error (MSE) to measure the numerical precision of the annotator, which is commonly used in video quality assessment (VQA) benchmarks to identify systematic bias or overly noisy raters~\cite{seshadrinathan2010study}. This metric effectively detects evaluators who have a biased offset (e.g., consistently rating too high or too low) or high variance compared to the group.
    \item \textbf{Ranking Consistency (Spearman's $\rho$):} We employ Spearman’s rank correlation coefficient to evaluate whether the annotator correctly orders the relative human-likeness of different clips, which is  
    % This is crucial because an annotator might have a strict scoring standard (high MSE) but still correctly distinguish that \textit{motion A} is more human-like than \textit{motion B} (high $\rho$).
    widely used in sports judging~\cite{zhou2024comprehensive}, and pairwise preference modeling~\cite{thurstone2017law}.
\end{itemize}

% By establishing data-driven thresholds ($\tau_{\mathrm{MSE}}$ at the 75th percentile and $\tau_{\rho}$ at the 25th percentile), we classify annotators based on their adherence to the collective distribution. We define \textbf{high-risk} annotators as those who fail \textit{both} criteria, meaning that they neither align with the group's numerical standard nor agree with the relative ranking logic. This conservative filtering strategy ensures we do not discard annotators who may simply be strict graders (high MSE) but consistent in ranking (high $\rho$).
Following established annotation filtering practice in VQA and human-rating literature~\cite{seshadrinathan2010study, snow2008cheap}, we determined the filtering thresholds using the 75th percentile of MSE and the 25th percentile of Spearman correlation. Annotators exceeding both thresholds simultaneously were labeled as \textbf{high-risk}, as this indicates they diverge from consensus both in absolute terms and in relative ranking. Medium-risk annotators violate only one of the two criteria and were retained but flagged for analysis.

The analysis identified 5 annotators as high-risk (MSE $\ge$ 1.41 and $\rho \le$ 0.50). As summarized in Tab.~\ref{tab:iac_summary}, removing these outliers significantly improved the dataset's internal consistency, with the mean MSE dropping from 1.1817 to 0.9764 and the mean Spearman correlation increasing from 0.5215 to 0.5457. This validation step confirms that our final annotations represent a stable and reliable consensus on human-likeness.

\begin{table}[t]
\centering
\caption{\textbf{Summary of annotator reliability based on Inter-Annotator Consistency (IAC).} High-risk annotators (MSE $\ge$ 1.41 and Spearman $\rho \le$ 0.50) were removed from the final rating pool.}
\vspace{2mm}
\resizebox{1\linewidth}{!}{
\begin{tabular}{lccc}
\toprule
\textbf{Annotator Group} & \textbf{Count} & \textbf{Mean MSE} & \textbf{Mean Spearman $\rho$} \\
\midrule
Retained Annotators & 25 & 0.9764 & 0.5457 \\
Removed Annotators  & 5  & 2.2081 & 0.4002 \\
\midrule
Total               & 30 & 1.1817 & 0.5215 \\
\bottomrule
\end{tabular}
}
\label{tab:iac_summary}
\end{table}

\begin{algorithm}[t]
\DontPrintSemicolon
\KwIn{Score matrix $S\in\mathbb{R}^{M\times N}$ where $s_{ij}$ is annotator $j$'s score on clip $i$.}
\KwOut{Retained annotator set $\mathcal{A}_{\mathrm{retain}}$ and removed set $\mathcal{A}_{\mathrm{remove}}$.}

\textbf{Compute clip-wise mean scores}\;
\For{$i\leftarrow 1$ \KwTo $M$}{
    $\bar{s}_i \leftarrow \frac{1}{N}\sum_{j=1}^{N} s_{ij}$\;
}

\textbf{Compute annotator MSE and Spearman correlation}\;
\For{$j\leftarrow 1$ \KwTo $N$}{
    $\mathrm{MSE}_j \leftarrow \frac{1}{M}\sum_{i=1}^{M} (s_{ij} - \bar{s}_i)^2$\;
    $\rho_j \leftarrow \mathrm{Spearman}(\{s_{1j},\dots,s_{Mj}\}, \{\bar{s}_1,\dots,\bar{s}_M\})$\;
}

\textbf{Compute filtering thresholds}\;
$\tau_{\mathrm{MSE}} \leftarrow \text{quantile}_{0.75}(\{\mathrm{MSE}_j\}_{j=1}^N)$\;
$\tau_{\rho} \leftarrow \text{quantile}_{0.25}(\{\rho_j\}_{j=1}^N)$\;

\textbf{Risk scoring and filtering}\;
\For{$j\leftarrow 1$ \KwTo $N$}{
    $R_j \leftarrow \mathbb{1}(\mathrm{MSE}_j \ge \tau_{\mathrm{MSE}}) + \mathbb{1}(\rho_j \le \tau_{\rho})$\;
    \uIf{$R_j = 2$}{
        mark annotator $j$ as \textbf{High-risk} (Remove)\;
    }
    \uElseIf{$R_j = 1$}{
        mark annotator $j$ as \textbf{Medium-risk} (Retain, flagged)\;
    }
    \Else{
        mark annotator $j$ as \textbf{Low-risk} (Retain)\;
    }
}

\Return $\mathcal{A}_{\mathrm{retain}} = \{j: R_j \le 1\},\quad \mathcal{A}_{\mathrm{remove}} = \{j: R_j = 2\}$\;

\caption{Inter-Annotator Consistency (IAC) Filtering Algorithm.}
\label{alg:iac_algo}
\end{algorithm}

% \subsection{Data Analysis on Human Imitating Humanoid}
% To reinforce the principle of the Motion Turing Test, we included a subset in the HHMotion dataset where human subjects intentionally imitated the movement patterns of humanoid robots. 
% % The primary objective of this subset was to generate ambiguous motion samples that blur the line between human and robotic behaviors, thereby increasing the difficulty of the evaluation and better reflecting the essence of the Motion Turing Test. 
% This subset contains 50 paired examples of human imitators and humanoid robot motions, with each motion clip rated by human annotators on a 0–5 scale and also evaluated by automated scoring methods.

% As shown in Table~\ref{tab:human_imitation_analysis}, human imitators generally receive intermediate scores that lie between the typical human and humanoid ranges. For instance, human imitators achieving an average human score of 3.2--4.0 are often rated closer to humanoid motions by the baseline predictor, highlighting the perceptual ambiguity of these motions. Moreover, the Gemini\_CoT\_Few\_Shot model demonstrates a consistent but more conservative trend, often underestimating the human-likeness of the imitated actions. Overall, this analysis confirms that the human-imitating-humanoid subset successfully introduces challenging motion samples, providing a robust testbed for both human and model evaluations under the Motion Turing Test framework.

\subsection{Data Analysis on Simulated Environment}
We further analyzed the subset of simulated humanoid motions, which consists of 243 samples spanning seven distinct action categories. Tab.~\ref{tab:sim_cate} reports the average human-likeness scores for each category, comparing human subjects and simulated humanoid motions. Overall, the simulated motions achieve higher scores than real humanoid robots, indicating that simulation allows for more precise or idealized motion execution. However, they still fall short of actual human performance in every category, highlighting the inherent gap between synthetic and natural human motion.

The analysis reveals that the discrepancy between simulated humanoids and real humans varies across actions. For example, the largest gap is observed in the \emph{jump} category (2.46 points), whereas \emph{waving} shows the smallest difference (0.35 points). This suggests that while simulations can effectively capture certain types of motions, they are less capable of replicating more complex or expressive movements that humans perform naturally. These findings emphasize that, although simulated data can serve as a useful proxy for evaluating motion algorithms, they cannot fully replace real human motion in benchmarks aiming to assess human-likeness.

\begin{table}[t]
\centering
\caption{\textbf{Human vs. Humanoid (simulated) motion quality comparison.}  
Simulated humanoids consistently score lower than humans, with the largest gaps appearing in high-dynamic actions such as \emph{jump} and \emph{boxing}. 
% Although simulation improves stability compared to real robots, it still falls short of replicating true human motion quality.
}
\resizebox{\linewidth}{!}{
\begin{tabular}{lccc}
\toprule
\textbf{Category} & \textbf{Human} & \textbf{Humanoid (sim)} & \textbf{Score Difference} \\
\midrule
jump         & 4.43 & 1.97 & 2.46 \\
boxing       & 3.76 & 2.41 & 1.35 \\
run          & 3.73 & 2.45 & 1.28 \\
kicking ball  & 3.93 & 2.70 & 1.23 \\
kungfu       & 3.60 & 2.47 & 1.13 \\
dance        & 3.47 & 2.50 & 0.97 \\
waving       & 3.70 & 3.35 & 0.35 \\
\bottomrule
\end{tabular}
}
\label{tab:sim_cate}
\end{table}

\section{More Details on Motion Turing Test Task}
\subsection{PTR-Net Model Details}
%Further technical details of the PTR-Net model architecture.

The Pose-Temporal Regression Network (PTR-Net) is designed as a lightweight yet effective architecture for the Motion Turing Test task, mapping a 3D pose sequence to a continuous human-likeness score. PTR-Net consists of three main components: a temporal encoder, a spatial–temporal graph convolution module, and an attention-based regression head. The complete pipeline is illustrated in Fig.~7 of the main paper.

\textbf{Temporal Encoder.} Given an input pose sequence $X=\{x_t\}_{t=1}^T$, a two-layer bidirectional LSTM is employed to capture long-range temporal dependencies across frames. The encoder outputs temporally enriched features $H_t \in \mathbb{R}^{2h}$ that retain both forward and backward contextual information, which is essential for modeling motion continuity and temporal smoothness.

\textbf{Spatial–Temporal Graph Convolution (ST-GCN).} The encoded sequence is reshaped into a graph representation where each node corresponds to a body joint, and edges represent human skeletal connections. A stack of ST-GCN blocks alternates between spatial graph convolutions and temporal convolutions to extract joint coordination patterns. Unlike conventional skeleton-based GCNs, PTR-Net adopts a parameter-free adjacency matrix, avoiding the need to learn fixed graph structures and enabling more flexible feature aggregation across joints and frames.

\textbf{Attention Pooling and Regression Head.} To emphasize motion segments that are most informative for judging human-likeness, a temporal attention mechanism is applied over the ST-GCN outputs. The weighted features are then passed into a lightweight MLP regression head that outputs a scalar human-likeness score. Formally, PTR-Net learns a mapping
\begin{equation}
    s = f_{\theta}(X),
\end{equation}
where $f_{\theta}$ denotes the network parameters and $s \in [0,5]$ is the predicted score.

\paragraph{Training Objective.} PTR-Net is trained with an L2 regression loss combined with a temporal smoothness regularization term:
\begin{equation}
    \mathcal{L} = \| \hat{s} - s^{*} \|_2^2 + \lambda \mathcal{L}_{\text{reg}},
\end{equation}
where $s^{*}$ is the ground-truth human-likeness score and $\hat{s}$ is the prediction. The regularization term $\mathcal{L}_{\text{reg}}$ penalizes excessive fluctuations across consecutive predictions, encouraging stability and consistency in the output scores.

Additional implementation details, hyperparameters, and network configurations are provided in the following sections of the supplementary material.

\subsection{Evaluation Metrics Definitions}

To systematically quantify the alignment between model predictions and human evaluations, we adopt three complementary evaluation metrics: Mean Absolute Error (MAE), Root Mean Squared Error (RMSE), and Spearman’s Rank Correlation~($\rho$). Their formal definitions and usage descriptions are provided below.

\textbf{Mean Absolute Error (MAE).}
MAE measures the absolute difference between the predicted scores and the human preference annotations, defined as:
\begin{equation}
\text{MAE} = \frac{1}{N}\sum_{i=1}^{N}|\hat{s}_i - s_i^*|,
\end{equation}
where \(\hat{s}_i\) and \(s_i^*\) denote the predicted and human scores for the \(i\)-th motion sequence, respectively.
A lower MAE indicates closer numerical alignment to human judgments.

\textbf{Root Mean Squared Error (RMSE).}
RMSE provides a more penalized metric for large deviations, given by:
\begin{equation}
\text{RMSE} = \sqrt{\frac{1}{N}\sum_{i=1}^{N}(\hat{s}_i - s_i^*)^2}.
\end{equation}
Compared with MAE, RMSE emphasizes stability and robustness by amplifying large prediction errors.

\textbf{Spearman’s Rank Correlation (\(\rho\)).}
Spearman’s $\rho$ measures the monotonic consistency between model-predicted rankings and human-provided rankings. We also compute Spearman’s rank correlation to evaluate monotonic consistency between model predictions and human annotations:
\begin{equation}
\rho = 1 - \frac{6\sum_i d_i^2}{N(N^2-1)},
\end{equation}
where \(d_i\) is the rank difference between predicted and annotated scores.
A higher \(\rho\) indicates that the model better preserves human-like relative ordering across motion samples.

\begin{figure*}[t]
    \centering
    \includegraphics[width=0.8\linewidth]{figs/prompt.png}
    \caption{\textbf{Prompt used for VLM-based human-likeness evaluation.}}
    \label{fig:vlm_prompt}
\end{figure*}

\begin{figure*}[t]
    \centering
    \includegraphics[width=0.8\linewidth]{figs/vlm_example.png}
    \caption{\textbf{VLM evaluation results on two unseen test videos.}}
    \label{fig:vlm_examples}
\end{figure*}

\subsection{Training Details}
%Specific training details for the PTR-Net baseline model

For the Motion Turing Test task, we train our proposed PTR-Net baseline exclusively on the HHMotion dataset. 
% All SMPL-X sequences are first normalized to a fixed length using linear temporal interpolation and processed into joint coordinate representations before being fed into the network. 
All the SMPL-X sequences are zero-padded to a maximum fixed length and processed into joint coordinate representations. A corresponding binary mask is generated for each sequence to ensure that the network ignores the padded regions during computation.
The human-likeness scores (ranging from 0 to 5) are normalized $[0, 1]$ for training stability. We partition the dataset into training and testing sets with a ratio of 80\% and 20\%, respectively.
% During training, we use the Adam optimizer with an initial learning rate of \(1\times10^{-3}\) and a batch size of 32. The model is trained for 200 epochs with early stopping based on the validation MAE.
The  model is trained for 500 epochs using the AdamW optimizer with an initial learning rate of $1\times10^{-3}$ and a weight decay of $1\times10^{-4}$. 
To make the model more robust to diversity in motion, data augmentation techniques like temporal jittering and joint-level Gaussian noise are used.

For comparison, we additionally evaluate two representative LLMs, Gemini-2.5 Pro~\cite{comanici2025gemini} and Qwen3-VL-Plus~\cite{bai2023qwen}. Both models process each SMPL-X motion clip as a video sequence input and output a human-likeness score following the same evaluation protocol as our baseline.

\section{Prompts for VLM Evaluation}
\label{sec:vlm_prompt}

\subsection{Evaluation Prompts}
To ensure a fair and reproducible evaluation of motion human-likeness, we design a structured prompt for the VLM. The prompt explicitly instructs the model to assess the human-likeness of a motion sequence represented by an SMPL-X model, based solely on kinematic information without any texture, facial details, or appearance cues.

Specifically, the VLM is first required to determine whether the motion belongs to upper-lower limb movement or full-body movement. Then instructed to evaluate the motion quality from three aspects: (1) posture fluency, (2) movement coordination, and (3) core stability. Based on these criteria, the model provides a comprehensive human-likeness score on a 0-5 scale, where 5 indicates indistinguishable from real human motion and 0 indicates completely robotic motion.

To reduce ambiguity and improve consistency, we provide six example videos in the prompt, each paired with a reference output including both a score and a detailed explanation. The VLM is instructed to follow the same format when evaluating a new input video. Fig.~\ref{fig:vlm_prompt} shows the complete prompt used in our experiments.

\subsection{Cases of VLM Evaluation}
\label{sec:vlm_testcases}

We present two representative test cases evaluated by the VLM PA-CoT instructions in Fig.~\ref{fig:vlm_examples}. In the first case, although the overall posture is natural and the core remains stable, slightly rigid head movements reduce coordination, leading to a score of 3. In the second case, the posture and balance appear highly human-like, but overly uniform timing and amplitude introduce subtle robotic characteristics, resulting in a score of 4.

\section{Limitations and Future Work}
While the proposed HHMotion dataset and the Motion Turing Test benchmark provide a rigorous foundation for evaluating the human-likeness of humanoid robots, we acknowledge several limitations in our current work that point towards promising directions for future research.

\textbf{Demographic Diversity of Annotators.} To ensure annotation consistency and quality control, our evaluation was primarily conducted in a laboratory setting with 30 university students and researchers (aged 20–30). While this provides a stable baseline for the Motion Turing Test, we acknowledge that this demographic may not fully represent the perceptual thresholds of broader populations, such as children or the elderly. Future iterations could employ crowdsourcing to verify the generalization of our human-likeness scores across diverse age groups and backgrounds.

\textbf{Kinematic Structure Mismatch.} Although we employed a rigorous manual cross-validation pipeline to filter reconstruction errors, mapping diverse humanoid robots to the human SMPL-X topology inevitably introduces minor failures that influence the evaluation. Future work could incorporate multi-view reconstruction and IMU-based validation to further strengthen reliability.

\section{Data Privacy and IRB}
This study, which involves the collection and processing of human motion data, was reviewed and approved by the Institutional Review Board (IRB). The online video data utilized in the HHMotion dataset were sourced from publicly accessible online platforms (e.g., YouTube) and are used strictly for non-commercial research purposes. We do not claim any copyright over the original video materials; all rights are retained by their respective creators.

To rigorously protect privacy, all individuals in the videos are anonymized. This process involves the full masking of faces and any other personally identifiable information (PII). The dataset to be publicly released consists solely of these anonymized video clips and their corresponding SMPL-X representations, ensuring that individual identities are safeguarded.

For videos involving volunteers, informed consent was obtained, authorizing the use of their data for research purposes. All annotations were conducted exclusively for academic research, in compliance with prevailing ethical standards in the field of human motion analysis.

\begin{figure*}[t]
    \centering
    \includegraphics[width=1\linewidth]{figs/15action_humanoid.png}
    \caption{\textbf{Fifteen humanoid motion categories.} This figure illustrates the full set of 15 action categories captured from real-world and simulated humanoid robots in HHMotion, covering both sport and daily motions.}
    \label{fig:15action_humanoid}
\end{figure*}

\begin{figure*}[t]
    \centering
    \includegraphics[width=1\linewidth]{figs/15action_human.png}
    \caption{\textbf{Fifteen human motion categories.} The corresponding 15 action categories were collected from human subjects, providing a comprehensive reference of natural human motion patterns for evaluating human-likeness.}
    \label{fig:15action_human}
\end{figure*}

% \section{Rationale}
% \label{sec:rationale}
% % 
% Having the supplementary compiled together with the main paper means that:
% % 
% \begin{itemize}
% \item The supplementary can back-reference sections of the main paper, for example, we can refer to \cref{sec:intro};
% \item The main paper can forward reference sub-sections within the supplementary explicitly (e.g. referring to a particular experiment); 
% \item When submitted to arXiv, the supplementary will already included at the end of the paper.
% \end{itemize}
% % 
% To split the supplementary pages from the main paper, you can use \href{https://support.apple.com/en-ca/guide/preview/prvw11793/mac#:~:text=Delete%20a%20page%20from%20a,or%20choose%20Edit%20%3E%20Delete).}{Preview (on macOS)}, \href{https://www.adobe.com/acrobat/how-to/delete-pages-from-pdf.html#:~:text=Choose%20%E2%80%9CTools%E2%80%9D%20%3E%20%E2%80%9COrganize,or%20pages%20from%20the%20file.}{Adobe Acrobat} (on all OSs), as well as \href{https://superuser.com/questions/517986/is-it-possible-to-delete-some-pages-of-a-pdf-document}{command line tools}.
